# Supplementary material for: Improving Scientific Document Retrieval with Concept Coverage-based Query Set Generation
Source: arXiv:2502.11181 source file (2025-02-16)
Supplement: Supplementary file 1 [file 080Appendix.tex]

\section{Appendix}
